# Supplementary material for: Crystallization and vitrification of electrons in a glass-forming charge liquid
Source: arXiv:1612.01804 source file (2017-10-05)
Supplement: Supplementary file 1 [file aal3120_Sasaki_SM.pdf]

# Materials and Methods

## Single crystal growth

Single crystals of the monoclinic $\theta_m$-(BEDT-TTF)$_2$TlZn(SCN)$_4$ were grown by the electrochemical oxidation method. The typical size of the crystals used for the resistivity, noise spectroscopy, optical conductivity, and specific heat measurements was ~ 0.1 mm × 1 mm × 0.3 mm. For the X-ray diffraction measurements, smaller crystals (~ 0.03 mm × 0.3 mm × 0.1 mm) were selected.

## Construction of time–temperature–transformation (TTT) diagram

The resistivity measurements were carried out with a current flow along the *b* axis. The electrical contacts were made using carbon paste. The time–temperature–transformation (TTT) diagram was constructed from the time-dependent resistivity change during the charge crystallization process at the various temperatures. The experimental procedure is as follows; first, the sample was cooled rapidly (>50 K/min) down to 50 K from the initial temperature of 200 K, and then heated up to each target temperature at a rate of 50 K/min, and finally held at the target temperature during each measurement.

## Noise spectroscopy, optical conductivity, X-ray diffraction, and specific heat measurements

The noise measurements were performed by a standard five-probe method including a center ground terminal (*39*). Thereby, the sample forms a part of a Wheatstone bridge circuit in order to cancel out the constant voltage offset between the two voltage terminals. A sinusoidal current with an operating frequency of 997 Hz was applied along the *b* axis. The voltage signal was detected by a lock-in amplifier (SR830) and processed by a spectrum analyzer (Agilent 35670A). The experiment was carried out above $T_m$ = 170 K, because the charge crystallization process prevents measurements in the supercooled charge-liquid state.

The polarized optical conductivity measurements were carried out with a Fourier transform microscope spectrometer in the range of 600–8000 cm$^{-1}$. A synchrotron radiation light source at BL43IR in SPring-8 was used. The optical conductivity was

calculated through a Kramers–Kronig (KK) transformation from the optical reflectivity determined by comparison with a gold thin film evaporated on the sample surface.

The X-ray diffraction measurements were performed by using a synchrotron radiation source ($\lambda = 1.0$ Å) at the Photon Factory (PF) BL-8A in the High Energy Accelerator Research Organization (KEK). The diffraction data were collected on an Imaging plate system (Rigaku). The oscillation angle of each photograph was 4 or 5°.

The specific heat was measured by the differential thermal analysis (DTA) method in the heating process with a sweeping rate of 0.5 K/min after slow cooling below the CO transition temperature.

## Supplementary Text

### Section I. Critical cooling rate for charge-glass formation

In $\theta$-(BEDT-TTF)$_2MM'$(SCN)$_4$ ($M$ = Tl, Rb, Cs, $M'$ = Zn, Co), there are two crystal forms with orthorhombic ($I$222) and monoclinic ($C$2) symmetries (*6*, *7*). Figure S1A and B shows the 2D molecular arrangement of the BEDT-TTF layer for the orthorhombic $\theta_o$-type system and the monoclinic $\theta_m$-type system, respectively. The intermolecular transfer integrals (the nearest-neighbor Coulomb interactions) are given by $t_1$ ($V_1$) and $t_2$ ($V_2$) in the $\theta_o$-type system and by $t_1$ ($V_1$), $t_2$ ($V_2$), and $t_2'$ ($V_2'$) in the $\theta_m$-type system. It should be noted that $t_2 \approx t_2'$ and $V_2 \approx V_2'$ for the $\theta_m$-type system (*6*, *40*). While the $\theta_o$-type salts exhibit the horizontal CO transition, the $\theta_m$-type salts show the diagonal CO transition (*16*). As discussed in Ref. 14, the material dependence of the CO transition temperature and the critical cooling rate for charge-glass formation in the $\theta_o$-type salts can be understood in terms of the anisotropy of the triangular lattice, $V_2/V_1$ (Fig. S1, C and D). With increasing $V_2/V_1$ (that is, with increasing the degree of geometrical frustration of the triangular lattice), the CO transition temperature and the critical cooling rate decrease, indicating that geometrical charge frustration between $V_1$ and $V_2$ plays an important role for the charge-glass formation in the $\theta_o$-type salts. Here, we plot the critical cooling rate for $\theta_m$-TlZn obtained in this study in Fig. S1D. In spite of the smaller value of $V_2/V_1$, the critical cooling rate of $\theta_m$-TlZn is slower than that of $\theta_o$-TlCo, suggesting different mechanisms of charge-glass formation between these two systems.

## Section II. Electron–lattice coupling in $\theta$-type compounds

Previous theoretical studies based on the extended Hubbard model (EHM) including electron–phonon coupling on a triangular lattice (*17*) have pointed out that the lattice degrees of freedom play an important role for reducing the geometrical charge frustration in the orthorhombic $\theta_o$-type compounds. Indeed, the orthorhombic $\theta_o$-RbZn and $\theta_o$-TlCo show a large lattice deformation at the CO transition temperature, suggesting the strong electron–lattice coupling. By contrast, in the monoclinic $\theta_m$-TlZn, the electron–lattice coupling is very weak compared to the orthorhombic $\theta_o$-type compounds, as confirmed by specific heat measurements. Figure S2A shows the relative change in the specific heat divided by temperature $\Delta C/T$ at the CO transition in $\theta_m$-TlZn and $\theta_o$-TlCo. $\Delta C/T$ in $\theta_m$-TlZn is much smaller than that in $\theta_o$-TlCo. Figure S2B shows the entropy change $\Delta S$ at the CO transition for $\theta_m$-TlZn and $\theta_o$-TlCo. Because the charge disproportion ratio of both compounds is 0.85:0.15, the entropy change due to the electronic part is estimated to be 2.2 $\mathrm{JK^{-1}mol^{-1}}$ (*40*). In $\theta_m$-TlZn, the most part of $\Delta S$ can be accounted for by the electronic contribution. On the other hand, in $\theta_o$-TlCo, a large lattice contribution to $\Delta S$ is observed. These results indicate that the contribution of the lattice degrees of freedom to the CO formation in the monoclinic $\theta_m$-TlZn is much smaller than that in the orthorhombic $\theta_o$-type system; namely, $\theta_m$-TlZn is closer to a system where the observed effects are electronic in nature. This is in good agreement with the EHM, in which the diagonal and horizontal CO patterns are expected in the absence and presence of electron–phonon coupling, respectively (*17*).

## Section III. Extended Hubbard model and spinless fermion model

The ground-state properties of $\theta$-(BEDT-TTF)$_2X$ have been extensively studied by the EHM on an anisotropic triangular lattice (*17*, *22*, *40–45*). The Hamiltonian of the EHM in the absence of electron–phonon coupling is given by

$$\mathcal{H}_{\mathrm{EHM}} = \sum_{\langle i,j\rangle\sigma}\left(-t_{ij}c_{i\sigma}^{\dagger}c_{j\sigma} + \mathrm{h.c.}\right) + U\sum_i n_{i\uparrow}n_{i\downarrow} + \sum_{\langle i,j\rangle} V_{ij}n_i n_j, \qquad \text{(S1)}$$

where $c_{i\sigma}^{\dagger}$ ($c_{i\sigma}$) is the creation (annihilation) operator for a hole at the *i*-th site with spin $\sigma$ ($\uparrow$ or $\downarrow$), $n_i$ ($\equiv \sum_\sigma n_{i\sigma} \equiv \sum_\sigma c_{i\sigma}^{\dagger}c_{i\sigma}$) is the number operator, $t_{ij}$ and $V_{ij}$ are the transfer integrals and the intersite Coulomb interactions between the *i*-th and *j*-th sites, respectively, and $U$ is the on-site Coulomb repulsion. When $U \gg t_{ij}$, the EHM is compatible to the spinless fermion model (*t*-*V* model) that neglects the spin degrees of freedom. The Hamiltonian of the *t*-*V* model is given by

$$\mathcal{H}_{t-V} = \sum_{\langle i,j \rangle} \left( -t_{ij} f_i^\dagger f_j + \text{h.c.} + V_{ij} \tilde{n}_i \tilde{n}_j \right), \tag{S2}$$

where $f_i^\dagger$ $(f_i)$ is the creation (annihilation) operator for a spinless fermion at the *i*-th site and $\tilde{n}_i = f_i^\dagger f_i$ is the number operator. It has been well established that the classical ground states of the *t*-*V* model ($t_{ij} = 0$) on an isosceles triangle lattice are disordered owing to geometric frustration when $V_1 \geq V_2$ as discussed in the main text, whereas the vertical CO becomes a unique ground state for $V_1 < V_2$ (Fig. S3A) (*23*, *24*, *46*, *47*). For $V_1 > V_2$, the chain-striped states such as the horizontal and diagonal COs emerge owing to the geometric frustration between the two diagonal Coulomb interactions $V_2$ (see Fig. 3A in the main text), which is the case for $\theta_m$-TlZn. When $V_1 = V_2$, the ground states include the vertical-striped state (Fig. S3A), the chain-striped states (Fig. S3, B and C), and a three-sublattice state (Fig. S3D), all of which are degenerate. The last one has been discussed in terms of a "pin-ball liquid" (*23*). The orthorhombic $\theta_o$-type compounds may be categorized in this regime. Indeed, three-fold diffuse rods have been observed in $\theta_o$-RbZn (*10*, *11*, *48*) and $\theta_o$-CsZn (*12*, *49*, *50*), which are different from what is observed in $\theta_m$-TlZn.

## Section IV. Assignment of vibrational modes in optical conductivity

As shown in Fig. S4A, the BEDT-TTF molecule has three C=C stretching modes: two Raman-active modes $\nu_2(a_g)$ and $\nu_3(a_g)$, and one infrared-active mode $\nu_{27}(b_{1u})$. Figure S4B shows the optical conductivity spectra $\sigma_1(\omega)$ of $\theta_m$-TlZn for the polarization of $\boldsymbol{E} \parallel \boldsymbol{c}$ measured in the slow cooling process at various temperatures. As shown in Fig. S4C, several vibrational modes of the BEDT-TTF molecule have been observed in the range of 1350–1550 cm$^{-1}$. According to Ref. 16, a few peaks around 1400 cm$^{-1}$ can be ascribed to the $CH_2$ bending modes $\nu_{28}$ and $\nu_{45}$, and broad bands at 1455 cm$^{-1}$ and 1480 cm$^{-1}$ can be assigned to $\nu_{3\mathrm{N}}$ and $\nu_{2\mathrm{I}}$, respectively. The Raman-active $\nu_2$ and $\nu_3$ modes become infrared-active because of weak dimerization of the two face-to-face BEDT-TTF molecules along the *b* direction. When the system is conductive above $T_m$ = 170 K, a broad $\nu_3$ mode is observed at around 1300 cm$^{-1}$ (see the highlighted region in Fig. S4B). However, in the insulating state below $T_m$, an opening of the optical gap leads to a decrease in intensity of the $\nu_3$ mode (Fig. S4B). The largest band at 1420 cm$^{-1}$ corresponds to $\nu_{27\mathrm{I}}$, whereas a small band at 1515 cm$^{-1}$ is assigned to $\nu_{27\mathrm{N}}$. Usually, the $\nu_{27}$ mode is observed for the polarization along the long molecular axis of BEDT-TTF, namely, along the *a* axis in the case of $\theta_m$-TlZn.

However, the $\nu_{27}$ mode can be observed for the polarization along the $c$ direction in $\theta_m$-TlZn because the BEDT-TTF molecular long axis in $\theta_m$-TlZn is tilted by 20° within the $a$-$c$ plane (*16*). It should be noted that the $\nu_{27}$ mode corresponding to $BEDT\text{-}TTF^{+0.5}$ is not observed even at room temperature (if present, it should be located at 1468 $cm^{-1}$). This is because the $\nu_{27}$ mode of $BEDT\text{-}TTF^{+0.5}$ measured in the in-plane polarization is screened by the conduction electrons within the 2D BEDT-TTF layers above $T_m$. As shown in Fig. S4C, some of the vibrational modes become smeared by thermal fluctuations with increasing temperature. Especially, the intensity of the $\nu_{27\mathrm{N}}$ mode becomes too small to detect experimentally above ~ 100 K. This is because the IR intensity of the $\nu_{27}$ mode depends on the charge distribution $\rho_c$ on the BEDT-TTF molecule. Indeed, based on quantum chemical calculations using a density functional theory (DFT) analysis, the IR intensity of $\nu_{27}$ has been calculated for the $\rho_c = 1$ (ionic), $\rho_c = 0$ (neutral), and $\rho_c = 0.5$ molecules, and it has been confirmed that the intensity of $\nu_{27}$ becomes smaller with decreasing charge distribution on the molecule (*51*, *52*). Therefore, in this study, we utilized the $\nu_{27\mathrm{I}}$ mode to investigate the temperature evolution of charge disproportionation in $\theta_m$-TlZn. We note that the difference of the IR intensities of $\nu_{27\mathrm{I}}$ between the charge-crystal ($\rho_c = 0.84$) and charge-glass ($\rho_c = 0.83$) states is estimated to be 1.7% if we simply assume a linear dependence of the IR intensity of $\nu_{27\mathrm{I}}$ on the charge distribution between $\rho_c = 0.5$ and 1, which is much smaller compared to the experimentally obtained difference between the charge-crystal and charge-glass states (see Fig. 2G).

## Section V. Effective medium percolation theory

In this study, we used the generalized effective medium (GEM) equation (*32*) to obtain the time evolution of the CO volume fraction $\phi(t)$ from the resistivity. In general, in the early stage of the nucleation and growth process, a large number of nuclei of the crystalline phase are formed (Fig. S7A), and in the intermediate state, the individual nuclei grow into particles independently (Fig. S7B). Finally, crystal growth stops when the grain boundaries touch one another (Fig. S7C). In this situation, we can assume that each domain grows without interacting with neighboring ones, where the standard percolation picture describing a spatially uncorrelated mixture of two phases can be applied. The generalized effective medium (GEM) equation with two morphology parameters $\phi_0$ and $\mu$ is given by (*32*)

$$\frac{\phi(\sigma_l^{1/\mu}-\sigma_m^{1/\mu})}{\sigma_l^{1/\mu}+[\phi_0/(1-\phi_0)]\sigma_m^{1/\mu}}+\frac{(1-\phi)(\sigma_h^{1/\mu}-\sigma_m^{1/\mu})}{\sigma_h^{1/\mu}+[\phi_0/(1-\phi_0)]\sigma_m^{1/\mu}}=0, \quad \text{(S3)}$$

where $\phi$ is the volume fraction of the insulating component (namely, in our case, the CO volume fraction) and $\phi_0$ is the critical volume fraction at which the percolation path is closed by insulating CO domains. Here, $\sigma_h$ ($\sigma_l$) is the conductivity of the metallic (insulating) component, $\sigma_m$ is the conductivity of the medium itself, and $\mu$ is an exponent depending on the dimensionality. While $\sigma_l$ was measured in the slow heating process after slow cooling, $\sigma_h$ was obtained in the rapid cooling process. The values of $\phi_0$ and $\mu$ have been calculated by using numerical simulations for various 2D and 3D crystal lattices (*31*, *53*). For the 2D triangular lattice, $\phi_0$ and $\mu$ are estimated to be 0.66 (Ref. 53) and 1.31 (Ref. 31), respectively. By using these values, we obtained the time evolution of the CO volume fraction, $\phi(t)$, at the various temperatures (Fig. 4, B and C).

## Section VI. Time–temperature–transformation (TTT) diagram

The crystallization rate below the melting temperature $T_m$ in the TTT diagram can be described by the nucleation and growth process in a first-order phase transition of a liquid. Because the free energies of the crystal and liquid phases intersect at $T_m$, if crystallization is avoided by rapid cooling, a supercooled liquid state emerges, where the driving force for nucleation is caused by the difference in the free energy between crystal and liquid, $\Delta G = G_{\text{crystal}} - G_{\text{liquid}}$ (see Fig. S5A). In the supercooled liquid state, the crystallization rate is given by $I = \exp\left(-\frac{\Delta g(r=r^*)}{k_B T}\right) \times \exp(-\frac{G_m}{k_B T})$, where $\Delta g(r)$ is the change in the total Gibbs free energy caused by the nucleated crystalline phase, $G_m$ is the activation energy for translational diffusion, $r$ is the radius of the nucleus, $r^*$ is a critical radius, and $k_B$ is the Boltzmann's constant. The former is a thermodynamic term, and the latter is a kinetic term. $\Delta g(r)$ is given by $4\pi r^2\sigma - (4/3)\pi r^3 \Delta G$ (where $\sigma$ is the surface energy), which has a thermodynamic energy barrier of $(16/3)\pi\sigma^3/(\Delta G)^2$ at the critical radius $r^* = 2\sigma/\Delta G$ (see Fig. S5B). For nucleation, the nucleus is needed to overcome the thermodynamic energy barrier $\Delta g(r = r^*)$. Therefore, if we assume $\Delta G \propto \Delta T$, the thermodynamic term is proportional to $\exp(-\frac{1}{T(\Delta T)^2})$. On the other hand, the kinetic term is proportional to

$\exp(-\frac{1}{T})$. As a result, the crystallization rate $I \propto \exp\left(-\frac{1}{T(\Delta T)^2}\right) \times \exp(-\frac{1}{T})$ exhibits a maximum at a nose temperature $T_{\mathrm{nose}}$ (see Fig. S5C).

## Section VII. Comparison with time–temperature–transformation (TTT) and continuous heating transformation (CHT) diagrams

Figure S6A shows the relation between the resistivity of the sample, $\rho_m$, and the CO volume fraction, $\phi$, derived from the GEM equation (see Sec. V). For the 2D triangular lattice, the critical volume fraction $\phi_0$ at which the percolation path is closed by the insulating CO domains is estimated to be 0.66 (*53*). Indeed, $\rho_m(\phi)$ has an inflection point at $\phi_0$ (see Fig. S6A). To check the validity of the GEM equation for the estimation of $\phi(t)$ from the resistivity, we reexamined the charge crystallization process in $\theta_m$-TlZn by measuring the resistivity in the heating process with various sweeping rates after rapid cooling (Fig. S6B). This experimental procedure constructs a so-called continuous heating transformation (CHT) diagram. As shown in Fig. S6B, charge crystallization has been observed as an abrupt increase in resistivity. We defined the crystallization temperature $T_X$ as the onset temperature of the abrupt increase (see Fig. S6B). The obtained $T_X$ is plotted along with the TTT diagram in Fig. S6C, which shows that the critical volume fraction $\phi_0 \approx 0.66$ determined from the percolation theory coincides comparatively well with the value obtained from the CHT diagram. This result supports the validity of the GEM equation for the estimation of the CO volume fraction from the resistivity.

## Section VIII. Johnson–Mehl–Avrami–Kolmogorov (JMAK) and Ostwald ripening processes

In a general nucleation and growth process, the crystallization rate at a constant temperature below $T_m$ can be given by the Johnson–Mehl–Avrami–Kolmogorov (JMAK) equation, $\phi(t) = 1 - \exp(-kt^n)$, where $k$ and $n$ are the JMAK parameters (*33*) (see Fig. 4, D to F). The JMAK equation describes how the crystalline phase develops from the liquid phase. The initial slow crystallization rate can be attributed to the time to form a large number of nuclei of the crystalline phase (Fig. S7A). In the intermediate region, the crystallization rate strongly increases as the nuclei grow into particles (Fig. S7B). In the final stage of the nucleation and growth process, many

boundaries are formed, where crystal growth stops (Fig. S7C). In contrast, Ostwald ripening is a crystallization process in which larger crystal domains further grow at the expense of smaller ones (*54*) (Fig. S7, D to F). In general, atoms or molecules on surfaces of a crystal are less stable than those of the interior, which causes a surface energy loss on the crystal–liquid interface. Therefore, domains with a large radius, in which the proportion of the interfacial surface energy relative to the total free energy is small, are energetically favored as compared to smaller domains. In other words, the system prefers a rearrangement of crystal grain boundaries through the Ostwald ripening process in order to minimize the total surface area. Thus, the small domains dissolve and adsorb onto the larger domains. The moderate time evolution of $\phi(t)$ observed in the final stage of crystal growth for $\theta_m$-TlZn in the temperature range between the nose temperature and $T_g$ can be well described by the Ostwald ripening process, $\phi(t) = 1 - (1 + k't)^{-1/3}$, where $k'$ is a constant (*34*) (see Fig. 4E).

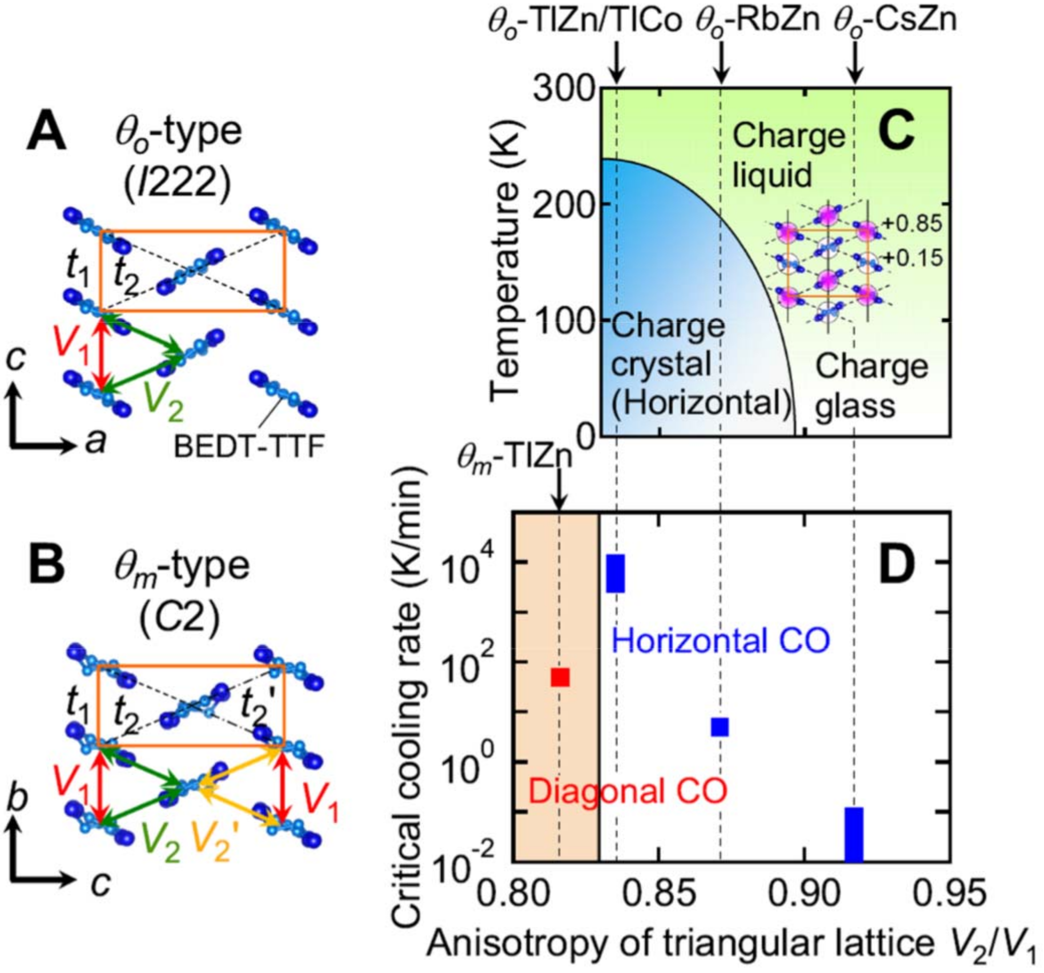


**Fig. S1. Orthorhombic and monoclinic types of *θ*-(BEDT-TTF)$_2$*X*.** (**A** and **B**) 2D conducting BEDT-TTF layers within (A) the *a*-*c* plane for the $\theta_o$-type salts and (B) the *b*-*c* plane for the $\theta_m$-type salts. The orange rectangles indicate the unit cell. (**C**) Generic phase diagram of the orthorhombic $\theta_o$-type materials as a function of $V_2/V_1$. An illustration of the horizontal CO pattern is shown in the inset. The orange rectangle represents the unit cell at the CO state. (**D**) Critical cooling rate for charge-glass formation as a function of $V_2/V_1$ for the monoclinic $\theta_m$-TlZn as well as the orthorhombic $\theta_o$-type materials.

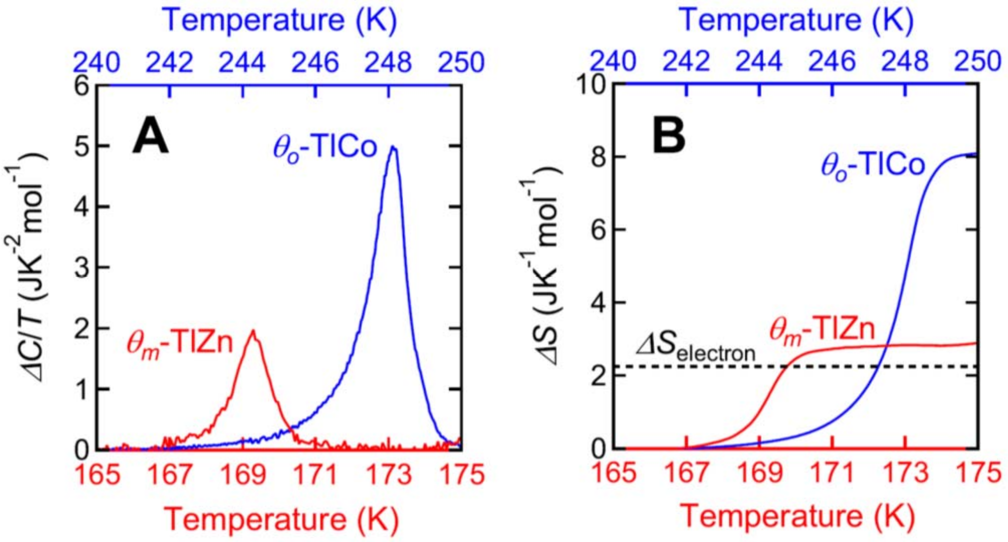


**Fig. S2. Specific heat measurements in $\theta_m$-(BEDT-TTF)$_2$TlZn(SCN)$_4$ and $\theta_o$-(BEDT-TTF)$_2$TlCo(SCN)$_4$.** (**A**) Relative change in the specific heat divided by temperature $\Delta C/T$ at the CO transition for $\theta_m$-TlZn (red, bottom axis) and $\theta_o$-TlCo (blue, top axis) measured in the heating process after slow cooling below $T_m$. (**B**) The corresponding entropy change $\Delta S$ for $\theta_m$-TlZn (red, bottom axis) and $\theta_o$-TlCo (blue, top axis). The dotted line indicates the electronic contribution to the entropy change when the charge disproportion ratio at the stripe COs is 0.85:0.15 (*40*).

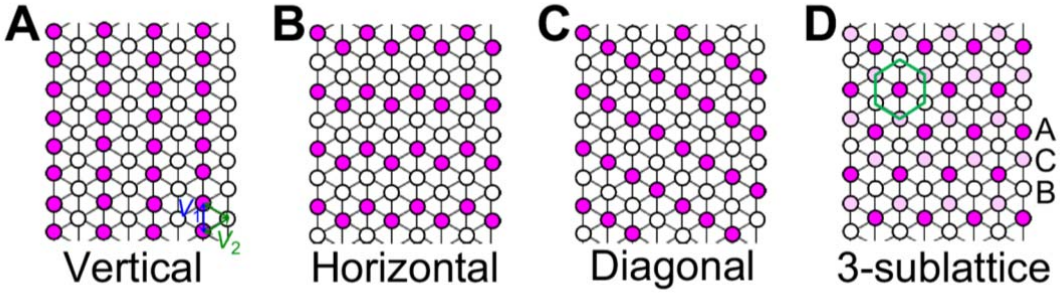


**Fig. S3. Charge configurations on the isosceles triangular lattice**. (**A**) vertical CO. (**B**) Horizontal CO. (**C**) Diagonal CO. (**D**) Three-sublattice CO. The magenta and white circles represent the charge-rich and charge-poor sites, respectively. In the three-sublattice structure, the sublattice A is filled by one hole ("pin"), the sublattice B is empty, and the sublattice C is randomly occupied by the remaining holes ("ball"). The green hexagon in (D) stands for the unit cell.

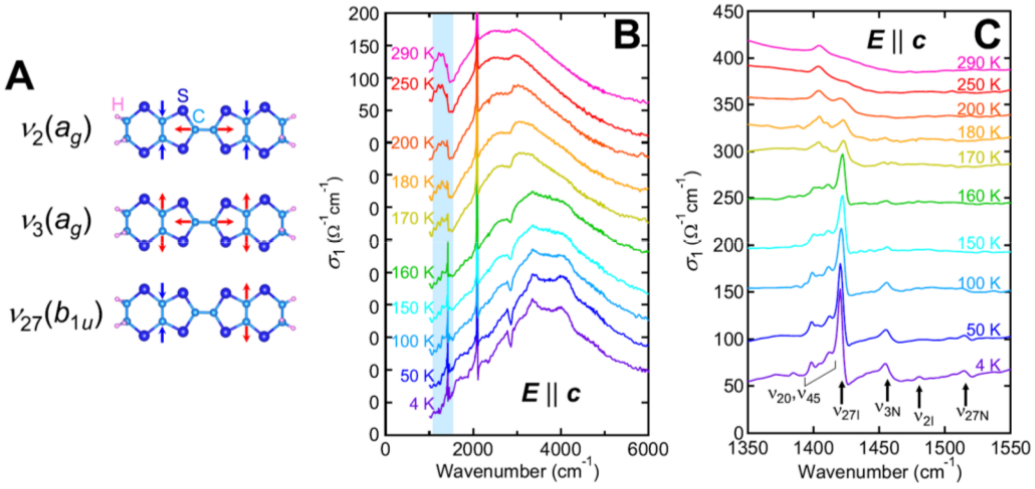


**Fig. S4. Optical conductivity measurements of $\theta_m$-(BEDT-TTF)$_2$TlZn(SCN)$_4$.** (**A**) Illustrations of three charge-sensitive C=C stretching modes of the BEDT-TTF molecule, $\nu_2(a_g)$, $\nu_3(a_g)$, and $\nu_{27}(b_{1u})$. The arrows indicate the shrinkage directions of the C=C bonds. (**B**) Polarized optical conductivity spectra (***E*** ∥ ***c***) of $\theta_m$-TlZn at various temperatures. The $\nu_3$ mode is located at the highlighted region. The sharp peak at approximately 2100 cm$^{-1}$ is the CN stretching mode of (SCN)$^{-1}$ in the anion layer. The dip-shaped anomaly around 2800 cm$^{-1}$ is ascribed to an overtone of the fundamental $\nu_3$ mode. The spectra are offset for clarity. (**C**) Expanded view of the polarized optical conductivity spectra (***E*** ∥ ***c***) of $\theta_m$-TlZn. The subscripts I and N represent the hole-rich and hole-poor sites, respectively.

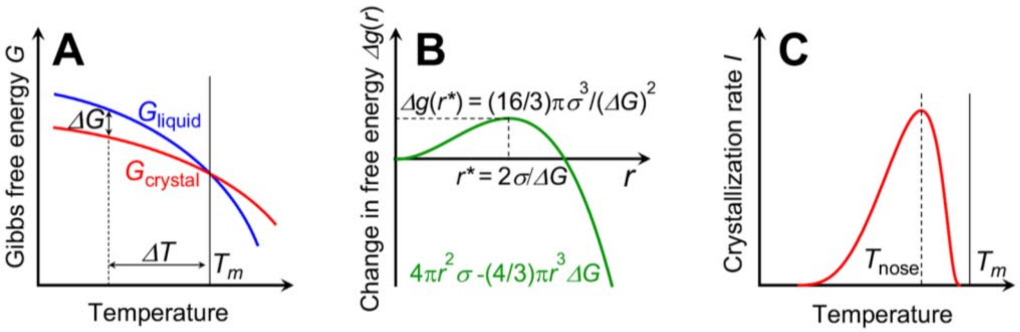


**Fig. S5. Nucleation and growth at a first-order liquid–crystal phase transition.** (**A**) Gibbs free energies of the liquid and crystal phases. (**B**) Change in the total free energy caused by the nucleated crystalline phase, $\Delta g(r)$. At the critical radius $r^* = 2\sigma/\Delta G$, $\Delta g(r^*) = (16/3)\pi\sigma^3/(\Delta G)^2$. (**C**) Crystallization rate derived from nucleation and growth theory. A characteristic peak structure appears at $T_{\mathrm{nose}}$.

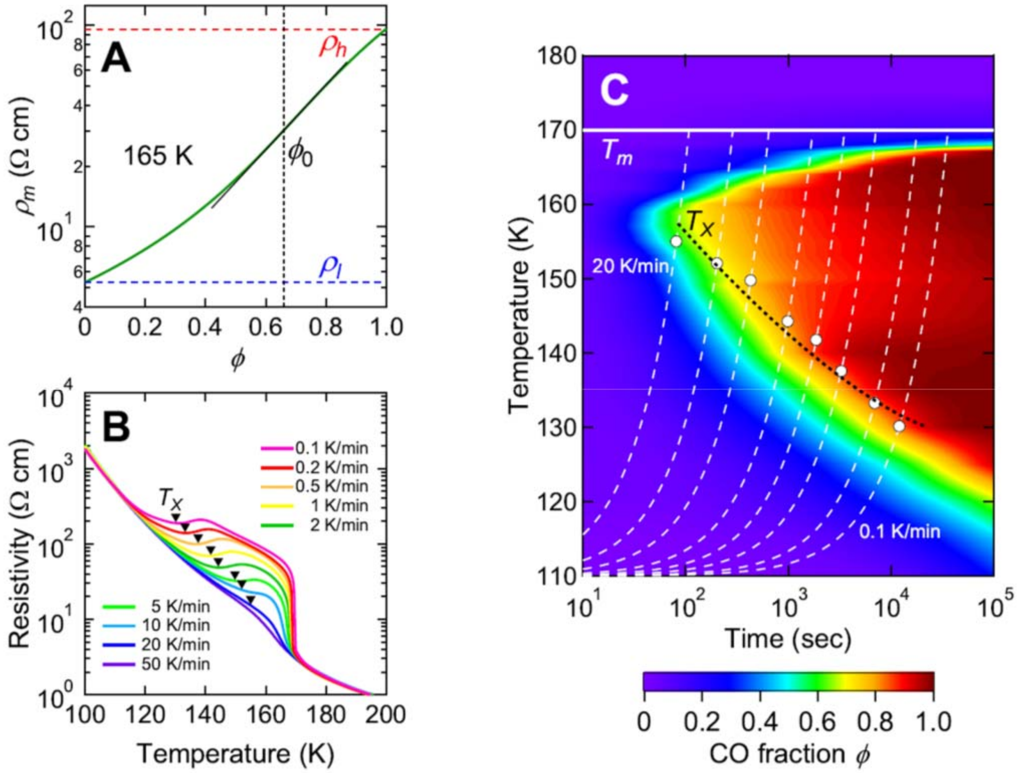


**Fig. S6. Time–temperature–transformation (TTT) and continuous heating transformation (CHT) diagrams.** (**A**) Log plot of $\rho_m$ as a function of $\phi$ at 165 K. The black solid line represents the slope of $\rho_m(\phi)$ at the reflection point $\phi_0$. Here, $\rho_l \equiv 1/\sigma_h$ and $\rho_h \equiv 1/\sigma_l$ (see Sec. V for the definitions of $\sigma_l$ and $\sigma_h$). (**B**) Temperature dependence of the resistivity measured in the heating process with various sweeping rates (0.1, 0.2, 0.5, 1, 2, 5, 10, 20, and 50 K/min) after rapid cooling. The inverted triangles indicate the crystallization temperature $T_X$ for each sweeping rate. (**C**) TTT diagram along with the CHT diagram. The white dashed curves represent the time dependence of the temperature for each resistivity measurement starting from 110 K, at which $\rho(T)$ in (B) begins to show a clear sweeping-rate dependence. The sweeping rates are 0.1–20 K/min from right bottom to left top. The elapsed time in the heating process of the CHT diagram with a sweeping rate of $R$ is defined as $t_R^{\mathrm{CHT}}(T) = t_R(T) - t_{R=50\ \mathrm{K/min}}(T)$. The black dotted curve is a guide to the eye.

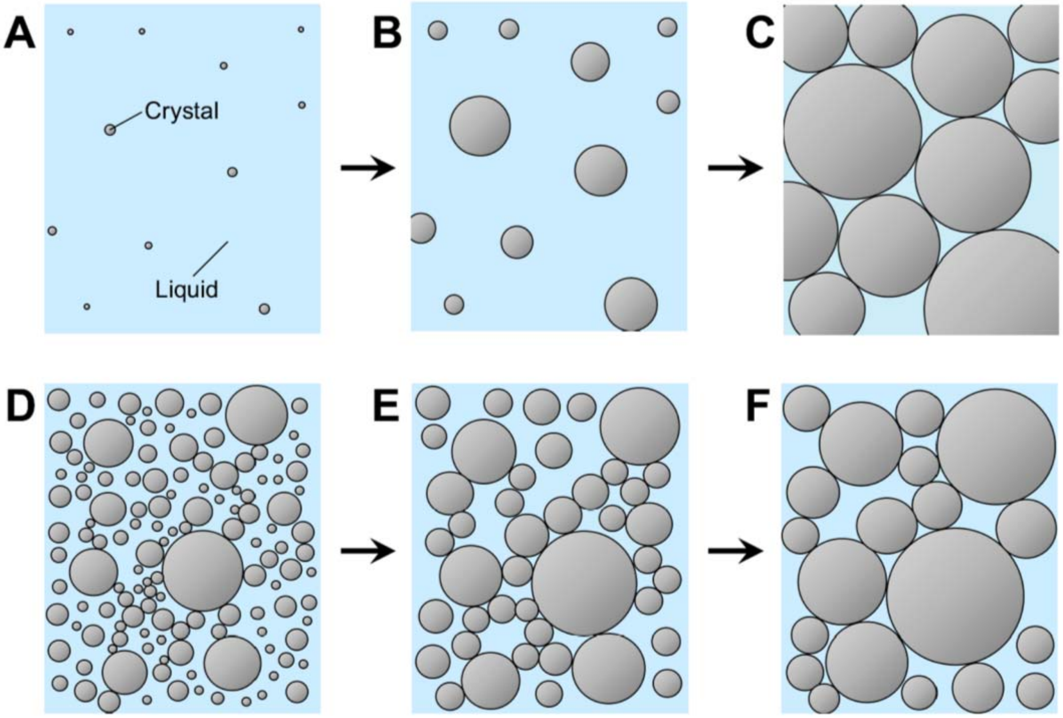


**Fig. S7. Johnson–Mehl–Avrami–Kolmogorov (JMAK) and Ostwald ripening processes.** (**A** to **C**) Illustrations of the nucleation and growth process described by the JMAK formula. The gray circles stand for crystal domains with various radii, while the blue area represents the liquid region. Time evolves from (A) to (C). (**D** to **F**) Illustrations of the Ostwald ripening process. Time evolves from (D) to (F). The smaller domains shrink, whereas the larger domains grow. The driving force comes from the difference in the total surface energy of the crystal–liquid interface among the domains, which arises from the difference in the radius of the domains. The system tends to minimize the interfacial free energy.

**References**


1. P. W. Anderson, Through the glass lightly. *Science* **267**, 1615–1616 (1995). doi:10.1126/science.267.5204.1615-e Medline

2. P. G. Debenedetti, F. H. Stillinger, Supercooled liquids and the glass transition. *Nature* **410**, 259–267 (2001). doi:10.1038/35065704 Medline

3. H. Shintani, H. Tanaka, Frustration on the way to crystallization in glass. *Nat. Phys.* **2**, 200–206 (2006). doi:10.1038/nphys235

4. T. Kawasaki, H. Tanaka, Formation of a crystal nucleus from liquid. *Proc. Natl. Acad. Sci. U.S.A.* **107**, 14036–14041 (2010). doi:10.1073/pnas.1001040107 Medline

5. C. A. Angell, Perspective on the glass transition. *J. Phys. Chem. Solids* **49**, 863–871 (1988). doi:10.1016/0022-3697(88)90002-9

6. H. Mori, S. Tanaka, T. Mori, A. Kobayashi, H. Kobayashi, Crystal structure and physical properties of M = Rb and Tl salts of (BEDT-TTF)2MM′$(SCN)_4$ [M′ = Co, Zn]. *Bull. Chem. Soc. Jpn.* **71**, 797–806 (1998). doi:10.1246/bcsj.71.797

7. H. Mori, S. Tanaka, T. Mori, Systematic study of the electronic state in θ-type BEDT-TTF organic conductors by changing the electronic correlation. *Phys. Rev. B* **57**, 12023–12029 (1998). doi:10.1103/PhysRevB.57.12023

8. F. Sawano, I. Terasaki, H. Mori, T. Mori, M. Watanabe, N. Ikeda, Y. Nogami, Y. Noda, An organic thyristor. *Nature* **437**, 522–524 (2005). doi:10.1038/nature04087 Medline

9. H. Seo, Charge ordering in organic ET compounds. *J. Phys. Soc. Jpn.* **69**, 805–820 (2000). doi:10.1143/JPSJ.69.805

10. M. Watanabe, Y. Noda, Y. Nogami, H. Mori, Transfer integrals and the spatial pattern of charge ordering in θ-$(BEDT\text{-}TTF)_2RbZn(SCN)_4$ at 90 K. *J. Phys. Soc. Jpn.* **73**, 116–122 (2004). doi:10.1143/JPSJ.73.116

11. F. Kagawa, T. Sato, K. Miyagawa, K. Kanoda, Y. Tokura, K. Kobayashi, R. Kumai, Y. Murakami, Charge-cluster glass in an organic conductor. *Nat. Phys.* **9**, 419–422 (2013). doi:10.1038/nphys2642

12. T. Sato, F. Kagawa, K. Kobayashi, K. Miyagawa, K. Kanoda, R. Kumai, Y. Murakami, Y. Tokura, Emergence of nonequilibrium charge dynamics in a charge-cluster glass. *Phys. Rev. B* **89**, 121102(R) (2014). doi:10.1103/PhysRevB.89.121102

13. T. Sato, F. Kagawa, K. Kobayashi, A. Ueda, H. Mori, K. Miyagawa, K. Kanoda, R. Kumai, Y. Murakami, Y. Tokura, Systematic variations in the charge-glass-forming ability of geometrically frustrated $\theta$-(BEDT-TTF)2$X$ organic conductors. *J. Phys. Soc. Jpn.* **83**, 083602 (2014). doi:10.7566/JPSJ.83.083602

14. H. Oike, F. Kagawa, N. Ogawa, A. Ueda, H. Mori, M. Kawasaki, Y. Tokura, Phase-change memory function of correlated electrons in organic conductors. *Phys. Rev. B* **91**, 041101(R) (2015). doi:10.1103/PhysRevB.91.041101

15. S. Mahmoudian, L. Rademaker, A. Ralko, S. Fratini, V. Dobrosavljević, Glassy dynamics in geometrically frustrated Coulomb liquids without disorder. *Phys. Rev. Lett.* **115**, 025701 (2015). doi:10.1103/PhysRevLett.115.025701 Medline

16. K. Suzuki, K. Yamamoto, K. Yakushi, Charge-ordering transition in orthorhombic and monoclinic single-crystals of $\theta$-(BEDT-TTF)$_2$TlZn(SCN)$_4$ studied by vibrational spectroscopy. *Phys. Rev. B* **69**, 085114 (2004). doi:10.1103/PhysRevB.69.085114

17. M. Udagawa, Y. Motome, Charge ordering and coexistence of charge fluctuations in quasi-two-dimensional organic conductors $\theta$-(BEDT-TTF)$_2$X. *Phys. Rev. Lett.* **98**, 206405 (2007). doi:10.1103/PhysRevLett.98.206405 Medline

18. J. Jaroszyński, D. Popović, T. M. Klapwijk, Universal behavior of the resistance noise across the metal-insulator transition in silicon inversion layers. *Phys. Rev. Lett.* **89**, 276401 (2002). doi:10.1103/PhysRevLett.89.276401 Medline

19. V. Dobrosavljević, D. Tanasković, A. A. Pastor, Glassy behavior of electrons near metal-insulator transitions. *Phys. Rev. Lett.* **90**, 016402 (2003). doi:10.1103/PhysRevLett.90.016402 Medline

20. M. D. Ediger, P. Harrowell, Perspective: Supercooled liquids and glasses. *J. Chem. Phys.* **137**, 080901 (2012). doi:10.1063/1.4747326 Medline

21. T. Yamamoto, M. Uruichi, K. Yamamoto, K. Yakushi, A. Kawamoto, H. Taniguchi, Examination of the charge-sensitive vibrational modes in bis(ethylenedithio)tetrathiafulvalene. *J. Phys. Chem. B* **109**, 15226–15235 (2005). doi:10.1021/jp050247o Medline

22. M. Naka, H. Seo, Long-period charge correlations in charge-frustrated molecular θ-(BEDT-TTF)$_2$X. *J. Phys. Soc. Jpn.* **83**, 053706 (2014). doi:10.7566/JPSJ.83.053706

23. C. Hotta, N. Furukawa, Strong coupling theory of the spinless charges on triangular lattices: Possible formation of a gapless charge-ordered liquid. *Phys. Rev. B* **74**, 193107 (2006). doi:10.1103/PhysRevB.74.193107

24. Y. Han, Y. Shokef, A. M. Alsayed, P. Yunker, T. C. Lubensky, A. G. Yodh, Geometric frustration in buckled colloidal monolayers. *Nature* **456**, 898–903 (2008). doi:10.1038/nature07595 Medline

25. See supplementary materials.

26. A. Hirata, L. J. Kang, T. Fujita, B. Klumov, K. Matsue, M. Kotani, A. R. Yavari, M. W. Chen, Geometric frustration of icosahedron in metallic glasses. *Science* **341**, 376–379 (2013). doi:10.1126/science.1232450 Medline

27. E. Dagotto, Complexity in strongly correlated electronic systems. *Science* **309**, 257–262 (2005). doi:10.1126/science.1107559 Medline

28. J. Schmalian, P. G. Wolynes, Stripe glasses: Self-generated randomness in a uniformly frustrated system. *Phys. Rev. Lett.* **85**, 836–839 (2000). doi:10.1103/PhysRevLett.85.836 Medline

29. R. Jamei, S. Kivelson, B. Spivak, Universal aspects of coulomb-frustrated phase separation. *Phys. Rev. Lett.* **94**, 056805 (2005). doi:10.1103/PhysRevLett.94.056805 Medline

30. K. Yoshimi, H. Maebashi, Coulomb frustrated phase separation in quasi-two-dimensional organic conductors on the verge of charge ordering. *J. Phys. Soc. Jpn.* **81**, 063003 (2012). doi:10.1143/JPSJ.81.063003

31. D. Stauffer, A. Aharony, *Introduction to Percolation Theory* (Taylor and Francis, ed. 2, 1994).

32. D. S. McLachlan, M. Blaszkiewicz, R. E. Newnham, Electrical resistivity of composites. *J. Am. Ceram. Soc.* **73**, 2187–2203 (1990). doi:10.1111/j.1151-2916.1990.tb07576.x

33. M. Avrami, Kinetics of phase change. I. General theory. *J. Chem. Phys.* **7**, 1103–1112 (1939). doi:10.1063/1.1750380

34. I. M. Lifshitz, V. V. Slyozov, The kinetics of precipitation from supersaturated solid solutions. *J. Phys. Chem. Solids* **19**, 35–50 (1961). doi:10.1016/0022-3697(61)90054-3

35. T. Konishi, H. Tanaka, Possible origin of enhanced crystal growth in a glass. *Phys. Rev. B* **76**, 220201(R) (2007). doi:10.1103/PhysRevB.76.220201

36. Y. Sun, L. Zhu, K. L. Kearns, M. D. Ediger, L. Yu, Glasses crystallize rapidly at free surfaces by growing crystals upward. *Proc. Natl. Acad. Sci. U.S.A.* **108**, 5990–5995 (2011). doi:10.1073/pnas.1017995108 Medline

37. Y. J. Kim, R. Busch, W. L. Johnson, A. J. Rulison, W. K. Rhim, Experimental determination of a time-temperature-transformation diagram of the undercooled $Zr_{41.2}Ti_{13.8}Cu_{12.5}Ni_{10.0}Be_{22.5}$ alloy using the containerless electrostatic levitation processing technique. *Appl. Phys. Lett.* **68**, 1057–1059 (1996). doi:10.1063/1.116247

38. E. B. Moore, V. Molinero, Structural transformation in supercooled water controls the crystallization rate of ice. *Nature* **479**, 506–508 (2011). doi:10.1038/nature10586 Medline

39. J. Müller, Fluctuation spectroscopy: A new approach for studying low-dimensional molecular metals. *ChemPhysChem* **12**, 1222–1245 (2011). doi:10.1002/cphc.201000814 Medline

40. T. Mori, Non-stripe charge order in the θ-phase organic conductors. *J. Phys. Soc. Jpn.* **72**, 1469–1475 (2003). doi:10.1143/JPSJ.72.1469

41. R. T. Clay, S. Mazumdar, D. K. Campbell, Charge ordering in θ-$(BEDT\text{-}TTF)_2X$ materials. *J. Phys. Soc. Jpn.* **71**, 1816–1819 (2002). doi:10.1143/JPSJ.71.1816

42. M. Kaneko, M. Ogata, Mean-field study of charge order with long periodicity in θ-$(BEDT\text{-}TTF)_2X$. *J. Phys. Soc. Jpn.* **75**, 014710 (2006). doi:10.1143/JPSJ.75.014710

43. H. Watanabe, M. Ogata, Novel charge order and superconductivity in two-dimensional frustrated lattice at quarter filling. *J. Phys. Soc. Jpn.* **75**, 063702 (2006). doi:10.1143/JPSJ.75.063702

44. K. Kuroki, The origin of the charge ordering and its relevance to superconductivity in θ-(BEDT-TTF)$_2$X: The effect of the Fermi surface nesting and the distant electron-electron interactions. *J. Phys. Soc. Jpn.* **75**, 114716 (2006). doi:10.1143/JPSJ.75.114716

45. S. Nishimoto, M. Shingai, Y. Ohta, Coexistence of distinct charge fluctuations in θ-(BEDT-TTF)$_2$X. *Phys. Rev. B* **78**, 035113 (2008). doi:10.1103/PhysRevB.78.035113

46. H. Wannier, Antiferromagnetism. The triangular Ising net. *Phys. Rev.* **79**, 357–364 (1950). doi:10.1103/PhysRev.79.357

47. R. M. F. Houtappel, Order-disorder in hexagonal lattices. *Physica* **16**, 425–455 (1950). doi:10.1016/0031-8914(50)90130-3

48. M. Watanabe, Y. Noda, Y. Nogami, H. Mori, Investigation of X-ray diffuse scattering in θ-(BEDT-TTF)$_2$RbM′SCN$_4$. *Synth. Met.* **135–136**, 665–666 (2003). doi:10.1016/S0379-6779(02)00769-5

49. M. Watanabe, Y. Nogami, K. Oshima, H. Mori, S. Tanaka, Novel pressure-induced 2$k_F$ CDW state in organic low-dimensional compound θ-(BEDT-TTF)$_2$CsCo(SCN)$_4$. *J. Phys. Soc. Jpn.* **68**, 2654–2663 (1999). doi:10.1143/JPSJ.68.2654

50. Y. Nogami, J.-P. Pouget, M. Watanabe, K. Oshima, H. Mori, S. Tanaka, T. Mori, Structural modulation in θ-(BEDT-TTF)$_2$CsM′(SCN)$_4$ [M′ = Co, Zn]. *Synth. Met.* **103**, 1911 (1999). doi:10.1016/S0379-6779(98)00616-X

51. A. Girlando, Charge sensitive vibrations and electron-molecular vibration coupling in bis(ethylenedithio)-tetrathiafulvalene (BEDT-TTF). *J. Phys. Chem. C* **115**, 19371–19378 (2011). doi:10.1021/jp206171r

52. A. Girlando, M. Masino, S. Kaiser, Y. Sun, N. Drichko, M. Dressel, H. Mori, Spectroscopic characterization of charge order fluctuations in BEDT-TTF metals and superconductors. *Phys. Status Solidi B* **249**, 953–956 (2012). doi:10.1002/pssb.201100722

53. V. A. Vyssotsky, S. B. Gordon, H. L. Frisch, J. M. Hammersley, Critical percolation probabilities (bond problem). *Phys. Rev.* **123**, 1566–1567 (1961). doi:10.1103/PhysRev.123.1566

54. J. H. Yao, K. R. Elder, H. Guo, M. Grant, Theory and simulation of Ostwald ripening. *Phys. Rev. B* **47**, 14110–14125 (1993). doi:10.1103/PhysRevB.47.14110 Medline
